# Supplementary material for: Finite Time Regret Bounds for Minimum Variance Control of Autoregressive Systems with Exogenous Inputs
Source: arXiv:2305.16974 source file (2023-05-26)
Supplement: Supplementary file 1 [file state_bound.tex]

\section{Bounding $\|y(t)\|$}\label{sec:bound_state}
\subsubsection{Lemma 5-(ii) of~\cite{lai1987asymptotically}} 
We begin by stating this result. Suppose there exists a $K>0$ such that for sufficiently large $t$ we have,
\al{
|u(t)| \le \min \left\{ K|y(t)| , C \right\}.\label{cond:1}
}
Moreover, whenever $t\notin \cI$ and $K|y(t)|< C$, we have
\al{
|y(t+1) - w(t)| \ll C.\label{cond:2}
}
Then we have,
\al{
|y(t)| \ll C,~\mbox{ for sufficiently large } t.
}
\proof Note that we have
\al{
|u(t)| \le C,~w(t) \le C_1.
}
Hence, for sufficiently large $i$, and time $n_{i+1} > t> n_i + m_i$ if $K|y(t)|< C$, then from~\eqref{cond:2} we have,
\al{
|y(t+1)| &\le |w(t)| + \delta^2 C \notag\\
& \le C_1 + \delta^2 C\notag \\
& \le 2\delta^2 C. \qquad (C_1 \ll C)
}
We will use induction to prove that when $i$ is sufficiently large, then the following holds for times $t$ satisfying $n_i + \frac{m_i}{3} <t < n_{i+1}$,
\al{
|u(t)| < \delta C, ~ |y(t+1)| < \delta^2 C.\label{eq:tpt}
}
~\eqref{eq:tpt} has already been shown for $n_i + \frac{m_i}{3} < t<n_i + m_i$ in Lemma 5-(i), (note that $|u(t)|\le C_1$ was assumed since the very beginning for $t\in\cI$). Next, consider time $s$ satisfying $n_{i+1} > s>n_i + m_i$, and assume that~\eqref{eq:tpt} holds for $n_i + \frac{m_i}{3} \le t\le s$. We will show that~\eqref{eq:tpt} also holds for time $t=s+1$. Consider,
\al{
K |y(s+1)| &\le K \delta^2 C \qquad (\mbox{ induction hypothesis }~\eqref{eq:tpt}) \\
& < C  \qquad (\mbox{ choose } \delta < \frac{1}{\sqrt{K}}),
}
which shows that the conditions for~\eqref{cond:2} are satisfied. Hence,~\eqref{cond:2} yields us
\al{
|y(s+2)| \le \delta^2 C.
}
It thus remains to show $|u(s+1)|< \delta \cdot C$. We have,
\al{
|u(s+1)| &\le K|y(s+1)| \qquad  (\mbox{from} ~~\eqref{cond:1})\notag\\
&\le K \delta^2 \cdot C \qquad (\mbox{ induction hypothesis }~\eqref{eq:tpt})  \notag\\
&\le \delta \cdot C (\mbox{ choose }\delta < \frac{1}{K}). 
}
This completes the induction, and hence proves that~\eqref{eq:tpt} holds.  

Thus, we have shown that for times $t\notin \cI$, we have $|u(t)|\ll C$. Also, $|u(t)|\ll C$ also holds for $t\in\cI$ by design~\eqref{ineq:bd1}. Hence, we have shown that 
\al{
|u(t)|\ll C,~\forall t.\label{ineq:u}
}
From~\eqref{ineq:bd2} we already have
\al{
|w(t)| \ll C,~ \forall t.\label{ineq:w}
}
Upon substituting~\eqref{ineq:u},~\eqref{ineq:w} into~\eqref{ineq:1}, we obtain the following,
\al{
|y(t)| \ll C~\forall t.\label{ineq:y}
}

\qed
