# Supplementary material for: Finite Time Regret Bounds for Minimum Variance Control of Autoregressive Systems with Exogenous Inputs
Source: arXiv:2305.16974 source file (2023-05-26)
Supplement: Supplementary file 2 [file lai_am.tex]

from 2.15 of \cite{lai1986asymptotically}
