# Supplementary material for: Finite Time Regret Bounds for Minimum Variance Control of Autoregressive Systems with Exogenous Inputs
Source: arXiv:2305.16974 source file (2023-05-26)
Supplement: Supplementary file 3 [file notation.tex]

\section{Notation}
$\mbf{0}$ is a vector consisting of all zeros.~If $M$ is a matrix, we let $\det(M)$ denote its determinant and $\Tr(M)$ denote its trace. For a vector $x$, we let $x'$ be its transpose.~If $x$ and $y$ are two vectors, we let $x\cdot y$ or $x'y$ denote their dot product.
