# Supplementary material for: Finite Time Regret Bounds for Minimum Variance Control of Autoregressive Systems with Exogenous Inputs
Source: arXiv:2305.16974 source file (2023-05-26)
Supplement: Supplementary file 4 [file rho_dep.tex]

\section{Regret Dependence upon $\rho$}\label{sec:rho_dep}
Note that
$$
\tau\ust_2 = \max\left\{\Bigg\lceil\frac{\log \br{\frac{B_u}{C_1 \|Y_0\|} }}{\log \rho} \Bigg\rceil ,0  \right\} \lesssim \log\br{1\slash \rho} .
$$

Also, $\tau\ust_3$ is the smallest value of $n$ that satisfies,
\al{
\left[ B_2 \times \frac{\log n}{\sqrt{n}} +  \sqrt{\frac{\log n}{n}} \right] \times \left[b_1\br{p+ 1 + \frac{C_1}{1-\rho}  \left\{1  +  \sum_{\ell=1}^{q} |b_\ell|   \right\} }\right] \le \frac{\delta^2_1}{2}.
}
Thus, 
$$
\tau\ust_3 \lesssim \br{\frac{1}{1-\rho}}^2.
$$
Also, $t\ust_4 \lesssim \frac{1}{\log \rho}$.
